# Supplementary material for: Improving Trustworthiness of AI Disease Severity Rating in Medical Imaging with Ordinal Conformal Prediction Sets
Source: arXiv:2207.02238 source file (2022-07-05)
Supplement: Supplementary file 1 [file supp.tex]

% This is samplepaper.tex, a sample chapter demonstrating the
% LLNCS macro package for Springer Computer Science proceedings;
% Version 2.21 of 2022/01/12
%
\documentclass[runningheads]{llncs}
\usepackage[T1]{fontenc}
% T1 fonts will be used to generate the final print and online PDFs,
% so please use T1 fonts in your manuscript whenever possible.
% Other font encondings may result in incorrect characters.
%
\usepackage{graphicx}
% Used for displaying a sample figure. If possible, figure files should
% be included in EPS format.
%
% If you use the hyperref package, please uncomment the following two lines
% to display URLs in blue roman font according to Springer's eBook style:
%\usepackage{color}
%\renewcommand\UrlFont{\color{blue}\rmfamily}
%
\begin{document}
%
% \title{Contribution Title\thanks{Supported by organization x.}}
%
\maketitle              % typeset the header of the contribution
\end{document}
